# Supplementary material for: Vortex lattice in two-dimensional chiral XY ferromagnets and the inverse Berezinskii-Kosterlitz-Thouless transition
Source: arXiv:2006.04915 source file (2020-12-23)
Supplement: Supplementary file 1 [file supp.pdf]

# Vortex lattice in two dimensional chiral XY-ferromagnets and inverse BKT transition
# Supplemtal Information

A.Costa[1,2] and M.B. Sturla[1,2]

[1] *Facultad de Ciencias Exactas, Universidad Nacional de La Plata, C.C. 67, 1900 La Plata, Argentina*
[2] *Instituto de Física de Líquidos y Sistemas Biológicos, CCT La Plata, CONICET*

*Vortex annihilation mechanism and effective charge separation*

The figure Fig. 1 shows the annihilation of only one vortex, in this case a positive vortex, by creation of one positive charge. The annihilation of only one vortex is, in principle, possible from the microscopical point of view, and a detailed energetic analysis is required to discard this possibility, since the topological restriction because of discreetness of the d.o.f. and finite size effect, translate into an energetic argument. Notoriously, on the other hand, this possibility is automatically ruled out in the effective theory because of the charge neutrality condition, and the topological restriction is immediately fulfilled.

Once the excited pair of opposite charges is created (see Fig. 2), at sufficient high temperature they can decouple as is illustrated in Fig. 3.

*Cumulant expansion*

In this section we give more details of the cumulant expansion that was used when mapping the system to the 2D neutral Coulomb gas.

When expressing the series of modified Bessel functions of the first kind we encountered terms of the form $\exp(\ln(I_n(\beta\mathcal{J})))$. Writing an integral representation of the Bessel functions and using a Taylor expansion these can be recast as

$$\begin{aligned} I_n(\beta\mathcal{J}) &= \frac{1}{\pi}\int_0^{\pi} d\omega e^{\beta\mathcal{J}\cos(\omega)}\cos(n\omega) = \\ &= I_0(\beta\mathcal{J})\left(1+\sum_{p=1}^{\infty}(-1)^p\frac{T_p(\beta\mathcal{J})}{(2p)!}n^{2p}\right) \end{aligned} \tag{1}$$

where

$$T_p(\beta\mathcal{J}) = \frac{1}{\pi I_0(\beta\mathcal{J})}\int_0^{\pi} e^{\beta\mathcal{J}\cos(\omega)}\omega^{2p}d\omega. \tag{2}$$

And the terms of the form $\exp\left(\ln(I_n(\beta\mathcal{J}))\right)$ present in the partition can be rewritten taking the logarithm at both sides of (1)

$$\begin{aligned} \exp\left(\ln(I_n(\beta\mathcal{J}))\right) &= \exp\left(\ln(I_0(\beta\mathcal{J})) + \ln(1+f(n))\right) \\ &= I_0(\beta\mathcal{J})\exp(\ln(1+f(n))) \end{aligned} \tag{3}$$

with $f(n) = \sum_{p=1}^{\infty}(-1)^p\frac{T_p(\beta\mathcal{J})}{(2p)!}n^{2p}$. An expansion of $\ln(1+f(n))$ as a power series in $n$ is needed an can be written as

$$\ln(1+f(n)) = \sum_{p=0}(-1)^p D_p(\beta\mathcal{J})\frac{n^{2p}}{(2p)!}. \tag{4}$$

Taking the derivative of both sides and comparing term by term on each side the first few $D_p$ are found to be

$$D_1 = T_1, \tag{5a}$$
$$D_2 = T_2 - T_1^2, \tag{5b}$$

and so on. Integration by parts in the definition of the $T_p(\beta\mathcal{J})$ functions gives a recursive relation that leads to the low temperature behaviour

$$T_p(\beta\mathcal{J}) \sim \frac{(2p-1)!!}{(\beta\mathcal{J})^p} + O((\beta\mathcal{J})^{-p-1}) \tag{6}$$

for $\beta\mathcal{J} \gg 1$.

*Coulomb gas mapping.–*

annhilation.pdf

one_vortex annhilation.pdf

FIG. 1. Illustrative: The figure shows a configuration in which only one vortex, a positive one, has been eliminated from the lattice, and the remaining vortex-antivortex lattice has not been affected; $D$ dominated regime.

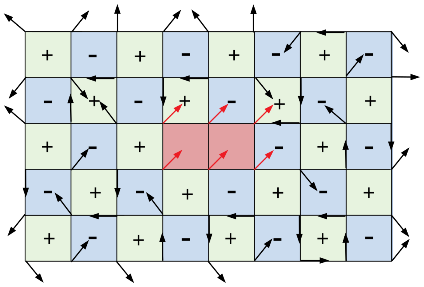

FIG. 2. Illustrative: opposite pseudo charge pair excitation corresponding to an annihilation of a positive vortex with a negative vortex; $D$ dominated regime.

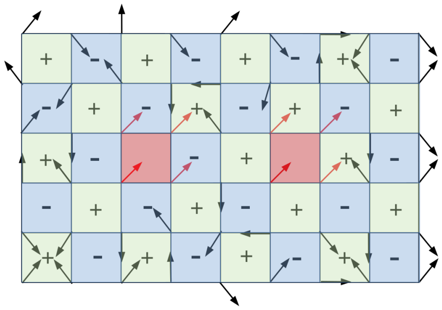

FIG. 3. Illustrative: Separation of the positive and negative pseudo charges; $D$ dominated regime.

In this section we give more details of the mapping that leads to the neutral Coulomb gas. We repeat here the same section presented in the main text with extra details. We start by noticing that $\mathcal{J}_\mu(\vec{r}_i)$ is independent of bond and lattice site, for the chosen $\varphi$ configuration, and representing $\varphi_\mu(\vec{r}_i)$ as a vector $\boldsymbol{\varphi}_i$ with components $\varphi_{\hat{x},i} = (-1)^{x_i+y_i}\varphi$ and $\varphi_{\hat{y},i} = (-1)^{x_i+y_i+1}\varphi$ on each site $i$, the partition function associated with the Hamiltonian (2) of the of the article can be written as:

$$Z = \int_{-\pi}^{\pi} \prod_j \frac{d\theta_j}{2\pi} \exp\left[\beta\mathcal{J}\sum_{i,\mu}\cos(\theta_i - \theta_{i+\mu} - \boldsymbol{\varphi}_i\cdot\hat{\mu})\right] \tag{7}$$

Expanding each exponential in series of Bessel functions[1], this partition function can be recast as:

$$Z = \sum_{\{n\}}\left(\prod_{i,\mu} I_{n_{i,\mu}}(\beta\mathcal{J})\exp\left[-in_{i,\mu}\boldsymbol{\varphi}_i\cdot\hat{\mu}\right]\right) \int_{-\pi}^{\pi}\left(\prod_j\frac{d\theta_j}{2\pi}\right)\exp\left[\sum_{i,\mu} in_{i,\mu}(\theta_i - \theta_{i+\mu})\right], \tag{8}$$

where $\{n\}$ represents a sum over all possible integers configurations, one $n_{i,\mu}$ per bond, and $I_n(\beta\mathcal{J})$ are the modified Bessel functions of first kind of order $n$. In this factorised way, integration over each angular variable can be done, and a theory on the discrete variable $n$, with the condition:

$$\boldsymbol{\Delta}\cdot\mathbf{n}_i = n_{i,x} - n_{i-\hat{x},x} + n_{i,y} - n_{i-\hat{y},y} = 0, \tag{9}$$

is obtained. Of course, this null discrete divergence condition can be immediately fulfilled by a discrte rotor $n_{j,\mu} = \epsilon_{\mu\nu}\Delta_\nu\phi_j$, where $\{\phi\}$ is a set of integers defined on the dual lattice, that it is the square lattice formed by the centre of the original plaquettes. Using $I_n(\beta\mathcal{J}) = \frac{1}{\pi}\int_0^\pi d\omega e^{\beta\mathcal{J}\cos(\omega)}\cos(n\omega)$ and expanding $\cos(n\omega)$,

$$Z = \sum_{\{\phi\}}\exp\left(\sum_{j,\mu}\sum_{p=1}^{\infty}\frac{D_p(\beta\mathcal{J})}{p!}(\Delta_\mu\phi_j)^{2p}\right) \times\exp\left[-\sum_{i,\mu} i\epsilon_{\mu\nu}\Delta_\nu\phi_i\boldsymbol{\varphi}_i\cdot\hat{\mu}\right], \tag{10}$$

where $D_p(\beta J)$ are the cumulant functions defined in[2], Introducing Dirac's deltas, $\sum_{k=-\infty}^{\infty}\delta(\phi-k) = \sum_{m=-\infty}^{\infty}e^{i2\pi m_j\phi_j}$, the sum over discrete variables can be turned into an integral of now continuous $\phi_j$ and,

$$Z = \int\mathcal{D}\phi\sum_{\{m\}}\exp\left[\sum_{j,\mu,p}(-1)^p\frac{D_p(\beta\mathcal{J})}{(2p)!}(\Delta_\mu\phi_j)^{2p} + i2\pi m_j\phi_j - i\epsilon_{\mu\nu}\Delta_\nu\phi_j\boldsymbol{\varphi}_j\cdot\hat{\mu}\right]. \tag{11}$$

Noticing that, since $\varphi_i$ change sign from site to site, the DM interaction can be rewritten as

$$-i\sum_i\epsilon_{\mu\nu}\Delta\phi_i\boldsymbol{\varphi}_i\cdot\hat{\mu} = -i\sum_i(-1)^{x_i+y_i}4\varphi\phi_i, \tag{12}$$

and that at sufficient low temperature we keep the lowest order in $T$. Since $D_p$ are of order $O((\beta\mathcal{J})^{2p-1})$ only the first $D_p$ is relevant and can be approximated by $D_1(\beta\mathcal{J}) = 1/\beta\mathcal{J} + O\left((\beta\mathcal{J})^{-2}\right)$, the low energy partition function can be written as:

$$Z = \int\mathcal{D}\phi\sum_{\{m\}}\exp\left[\sum_{\mu,j} -\frac{1}{2\beta\mathcal{J}}(\Delta_\mu\phi_j)^2 + i2\pi M_j\phi_j\right], \tag{13}$$

where $M_j = m_j - (-1)^{x_j+y_j}\frac{2\varphi}{\pi}$ has been introduced.

By Fourier transforming the fields $\phi_j = \frac{1}{(2\pi)^2}\int_{-\pi}^{\pi}d^2qe^{-i\vec{q}\cdot\vec{j}}\eta(\vec{q})$, $M_j = \frac{1}{(2\pi)^2}\int_{-\pi}^{\pi}d^2qe^{-i\vec{q}\cdot\vec{j}}l(\vec{q})$ and performing the Gaussian integrals, the partition function reads:

$$Z = \sum_{\{m\}}\exp\left[-\int_{-\pi}^{\pi}d^2q\frac{1}{2}\ln\left(\frac{2K(q)}{\pi}\right) + \frac{|l(q)|^2}{16K(q)\pi^2}\right]. \tag{14}$$

where $K(q) \simeq \frac{1}{2\beta\mathcal{J}\pi^2}\left(1 - \frac{1}{2}\sum_\mu\cos(\vec{q}\cdot\hat{\mu})\right)$ at sufficiently low temperatures. Transforming back to real

space the partition function reads

$$Z = Z^0 \sum_{\{m\}} \exp\left[-\frac{\beta\mathcal{J}}{8}\sum_{i,j} M_i V_{ij} M_j\right]. \quad (15)$$

where:

$$Z^0 = \exp\left[-\int_{-\pi}^{\pi} d^2q \frac{1}{2}\ln\left(\frac{2K(q)}{\pi}\right)\right] \quad (16)$$

$$V_{ij} = \int_{-\pi}^{\pi} d^2q \frac{e^{i\vec{q}(\vec{i}-\vec{j})}}{\left(1-\frac{1}{2}\sum_\mu \cos(\vec{q}\cdot\hat{\mu})\right)},$$

with $K(q)$ approximated by

$$K(q) = \frac{1}{2\beta\mathcal{J}\pi^2}(1-\frac{1}{2}\sum_\mu \cos(\vec{q}\cdot\hat{\mu})).$$

For small $|q|$ the potential reduces to the Coulomb gas potential, $V_{ij} \simeq 2\int d^2q e^{iq(i-j)}/|q|^2$, that after proper regularisation by imposing charge neutrality $\sum_i M_i = 0$ [3], leads to the low temperature partition function:

$$Z = Z^0 \sum_{\{m\}} \exp\left[\pi\beta\mathcal{J}\sum_{i,j} M_i \ln(|\mathbf{R}_i - \mathbf{R}_j|) M_j - \pi\beta\mathcal{J}\sum_l \left(\frac{1}{2}\ln(8)+\gamma\right) M_l^2\right]. \quad (17)$$

*Low temperature approximation of the helicty modulus*

We will obtain a low temperature approximation for the helicity modulus $\Upsilon$ in the extreme DMI regime where $J \to 0$ following Ohta and Jasnow[4]. We impose a long-wavelength “twist”, that has a wavelength $\lambda_0$, of the local short range order by defining a new set of variables $\theta'(\mathbf{r})$ given by

$$\theta(\mathbf{r}) = \theta'(\mathbf{r}) + \Phi(\mathbf{r}) \quad (18)$$

with $\Phi(\mathbf{r}) = k_0 x$ and $k_0 = 2\pi/\lambda_0$. A finite jump on the helicity modulus is expected in going from correlated to decorretated pahse, where the helicity modulus $\Upsilon$ is defined as:

$$\Upsilon \equiv \left.\frac{\partial^2 F(T,k_0)}{\partial k_0^2}\right|_{k_0=0}. \quad (19)$$

To calculate $\Upsilon$ we must then evaluate the free energy $F(T,k_0) = -T\ln(Z(\Phi,T))$ given by the partition function

$$Z = \int_{-\pi}^{\pi} \frac{\prod_j d\theta_j}{2\pi} \exp\left[\beta\mathcal{J}\sum_{j,\hat{\mu}} \cos\left(\theta'_j - \theta'_{j+\mu} - \boldsymbol{\varphi}_j\cdot\hat{\mu} + \Phi_j - \Phi_{j+\mu}\right)\right]. \quad (20)$$

The duality transformations we used in the previous section, that correspond to the $\Phi = 0$ case, can still be applied leading to

$$Z = \int \mathcal{D}\phi \sum_{\{m\}} \exp\left[H_0 + H_M + H_\Phi\right] \quad (21)$$

with

$$H_0 = \sum_{l,\mu,p} (-1)^p \frac{D_p(\beta\mathcal{J})}{(2p)!}(\Delta_\mu\phi_j)^{2p} \quad (22a)$$

$$H_\Phi = i\sum_l (\phi_{l+\hat{y}} - \phi_l)(\Phi_l - \Phi_{l+\hat{x}}) \quad (22b)$$

$$H_M = 2\pi i \sum_l M_l \phi_l \quad (22c)$$

For $\beta\mathcal{J} \gg 1$ the first few $D_p$ are given by

$$D_1 = \frac{1}{\beta\mathcal{J}}\left(1+\frac{1}{2\beta\mathcal{J}}\right) \quad (23a)$$

$$D_2 = (\beta\mathcal{J})^{-3} \quad (23b)$$

and the next $D_p$ are of order $O[(\beta\mathcal{J})^{2p-1}]$. As mentioned before, to obtain the helicity modulus we only need the free energy up to $O(k_0^2)$, so at sufficiently low temperatures we keep now the first two terms in $H_0$ giving

$$H_0 = -\frac{D_1(\beta\mathcal{J})}{2}(\Delta_\mu\phi_j)^2 + \frac{D_2}{4!}(\Delta_\mu\phi_j)^4. \quad (24)$$

Performing the Gaussian integrals by Fourier transforming the fields and treating the $D_4$ term as a perturbation, the partition function reads

$$Z = Z^0 \sum_{\{m\}} \exp\left(H(\{m\},\Phi)\right) \quad (25)$$

with

$$H(M,\Phi) = -\frac{1}{2D_2}\int_{\mathbf{k}} \frac{\sigma_{\mathbf{k}}\sigma_{-\mathbf{k}}}{f(\mathbf{k})} + \frac{D_4}{4!D_2^4}\int_{\mathbf{k}_1\mathbf{k}_2\mathbf{k}_3\mathbf{k}_4} U(\mathbf{k}_1,\mathbf{k}_2\mathbf{k}_3,\mathbf{k}_4)\sigma_{\mathbf{k}_1}\sigma_{\mathbf{k}_2}\sigma_{\mathbf{k}_3}\sigma_{\mathbf{k}_4} - \frac{6D_4}{4!D_2^3}\int_{\mathbf{k},\vec{q}} U(\mathbf{k},-\mathbf{k},\vec{q},-\vec{q})f(-\mathbf{k})\sigma_{\vec{q}}\sigma_{-\vec{q}} \quad (26)$$

where we introduced

$$f(\mathbf{q}) = \frac{1}{2}\sum_{\hat{\mu}} |1-e^{i\hat{\mu}\cdot\mathbf{q}}|^2, \quad (27)$$

$$\sigma_{\mathbf{q}} = 2\pi M(\mathbf{q}) - f(\mathbf{q})\Phi(\mathbf{q}), \quad (28)$$

$$V(\mathbf{q}_1,\mathbf{q}_2,\mathbf{q}_3,\mathbf{q}_4) = \delta(\mathbf{q}_1+\mathbf{q}_2+\mathbf{q}_3+\mathbf{q}_4)\sum_{\hat{\mu}}\prod_{i=1}^{4}\left(1-e^{i\mathbf{q}_i\cdot\hat{\mu}}\right) \quad (29)$$

and

$$U(\mathbf{k}_1, \mathbf{k}_2, \mathbf{k}_3, \mathbf{k}_4) = \frac{\frac{1}{2}V(\mathbf{q}_1, \mathbf{q}_2, \mathbf{q}_3, \mathbf{q}_4)}{\prod_{i=1}^4 f(\mathbf{k}_i)}. \tag{30}$$

Up to order $O(k_0^2)$ the free energy reads

$$\begin{aligned} -\ln(Z(\Phi))/\beta = -\frac{1}{\beta}\int_{\mathbf{k}} |\hat{\Phi}_k|^2 \hat{f}(\mathbf{k}) \\ \left(-\frac{1}{2D_1} - \frac{D_2}{4D_1^3}\int_{\vec{q}} \hat{V}(\mathbf{k},\vec{q}) + \frac{2\pi^2}{D_1^2}\frac{\langle |M_{\vec{q}}|^2\rangle}{f(\mathbf{k})}\right. \\ \left. + \frac{\pi^2 D_2}{D_1^4}\int_{\vec{q}} \hat{V}(\mathbf{k},\vec{q})\frac{\langle |M_{\vec{q}}|^2\rangle}{f(\vec{q})}\right) \end{aligned} \tag{31}$$

where we have defined

$$\hat{V}(\mathbf{k},\mathbf{q}) = f(-\mathbf{k})U(\mathbf{k},-\mathbf{k},\mathbf{q},-\mathbf{q})f(\mathbf{q}) \tag{32}$$

and

$$\hat{f}(\mathbf{k}) = |1 - e^{ik_x a}(1 - e^{-ik_y a})|^2 / f(\mathbf{k}). \tag{33}$$

we can identify directly $\Upsilon$ in (31) as

$$\begin{aligned} -\beta\Upsilon = \lim_{k_y\to 0}\lim_{k_x\to 0}\frac{\hat{f}(\mathbf{k})}{2k_x^2} \\ \left(-\frac{1}{D_1} - \frac{2D_2}{4D_1^3}\int_{\vec{q}} \hat{V}(\mathbf{k},\vec{q}) + \frac{4\pi^2}{D_1^2}\frac{\langle |M_{\vec{q}}|^2\rangle}{f(\mathbf{k})}\right. \\ \left. + \frac{2\pi^2 D_2}{D_1^4}\int_{\vec{q}} \hat{V}(\mathbf{k},\vec{q})\frac{\langle |M_{\vec{q}}|^2\rangle}{f(\vec{q})}\right). \end{aligned} \tag{34}$$

We note

$$\lim_{k_x\to 0}\frac{\hat{f}(\mathbf{k})}{k_x^2} = 1 \tag{35a}$$

$$\lim_{k_x\to 0}\int_q \hat{V}(\mathbf{q},\mathbf{k}) = \frac{1}{2} \tag{35b}$$

leading to

$$\begin{aligned} \beta\Upsilon = \frac{1}{D_1} + \frac{D_2}{4D_1^3} - \frac{4\pi^2}{D_1^2}\lim_{\mathbf{k}\to 0}\frac{\langle |M_{\mathbf{q}|^2}\rangle}{f(\mathbf{q})} \\ - \frac{2\pi^2 D_2}{D_1^4}\int_{\mathbf{q}}\frac{\langle |M_{\mathbf{q}}^2|\rangle}{f(\mathbf{q})}. \end{aligned} \tag{36}$$

Using the low temperature expansion (23) for $D_1$ and $D_2$,

$$\Upsilon/\mathcal{J} = 1 + 2\alpha - \gamma - \frac{1}{\beta\mathcal{J}}\left(\frac{1}{4} - 2\gamma\right) - 2\alpha\beta\mathcal{J} \tag{37}$$

where $\alpha = 2\pi^2 \lim_{\mathbf{k}\to 0}\frac{\langle |M_{\mathbf{q}}|^2\rangle}{f(\mathbf{q})}$ and $\gamma = 2\pi^2\int_{\mathbf{q}}\frac{\langle |M_{\mathbf{q}}|^2\rangle}{f(\mathbf{q})}$. The terms that contain $\alpha$ and $\gamma$ correspond to the contribution to $\Upsilon$ due to charge interactions and are functions of $\beta$. We can compute them by calculating the charge-charge correlation following José and Kadanoff[5]. Since we are dealing with a low energy expansion the dominant configurations we need to take into account are the ground state configuration and configurations with a single pair of excited charges. For the $D$ dominated regime the ground state configuration has zero charges while the lowest energy excitation is made up from a pair of charges $M_1 = -M_2 = 1$. We find for $\mathbf{R}_1 \neq \mathbf{R}_2$

$$\begin{aligned} \langle M(\mathbf{R}_1)M(\mathbf{R}_2)\rangle &= -2e^{-2\beta\epsilon_c}e^{-\beta\pi\ln(|\mathbf{R}_1-\mathbf{R}_2|/a)} \\ &= -2e^{-2\beta\epsilon_c}(|\mathbf{R}_1-\mathbf{R}_2|/a)^{-\beta\pi} \end{aligned} \tag{38}$$

and for $\mathbf{R}_1 = \mathbf{R}_2$

$$\langle M(\mathbf{R}_1)^2\rangle = 2e^{-2\beta\epsilon_c}\sum_{\mathbf{R}}(|\mathbf{R}-\mathbf{R}_1|/a)^{-\beta\pi}. \tag{39}$$

The charge-charge correlation function behaves as $\langle M(R_1)M(R_2)\rangle \sim e^{-\beta}$ so we can neglect the low temperature charge contributions to $\Upsilon$, hence

$$\Upsilon/D = 1 - \frac{T}{4D}. \tag{40}$$

For the XY model, which is in the limit $D/J \to 0$, the ground state configuration also has zero charge and the same result holds, though in this case we have $\mathcal{J} = J$ giving

$$\Upsilon/J = 1 - \frac{T}{4J}. \tag{41}$$

For any case where $J$ and $D$ are both non-zero the ground state is no longer made up from zero charges and we expect a non vanishing correlation $\langle |M(q)|^2\rangle$, and in turn, a non-zero $\alpha$ and $\gamma$ even at low temperatures.

[1] M. Abramowitz and I. A. Stegun, *Handbook of mathematical functions with formulas, graphs, and mathematical tables*, Vol. 55 (US Government printing office, 1948).

[2] Supplemental material; cumulant functions.
[3] A. M. Schakel, *Boulevard of broken symmetries: effective field theories of condensed matter* (World Scientific Publishing Company, 2008).
[4] T. Ohta and D. Jasnow, Physical Review B **20**, 139 (1979).
[5] J. V. José, L. P. Kadanoff, S. Kirkpatrick, and D. R. Nelson, Physical Review B **16**, 1217 (1977).
